# Supplementary material for: Serpens: A High Bandwidth Memory Based Accelerator for General-Purpose Sparse Matrix-Vector Multiplication
Source: arXiv:2111.12555 source file (2022-05-09)
Supplement: Supplementary file 1 [file appendix.tex]

\begin{tableA*}[tb]
\caption{Comparison with related sparse accelerators.}
  \label{table:comparison}
  \centering
  \begin{threeparttable}
  \begin{tabular}{ccccccccc}
    \hline
    & \textbf{Kernels} & \textbf{Mat. NNZ} & \textbf{Prob. Size} &
    \textbf{Throughput} & \textbf{FPGA} & \textbf{ASIC} & \textbf{Real Exe}& \textbf{1-for-all}\\
    \hline
    %\hline
    T2S-Tensor \cite{srivastava2019t2s} & Dense MM, MV, etc\tnote{1} & $2\times10^3$ & - &
    738 GFLOP/s & \textbf{Yes} & No & \textbf{Yes} & No \\
    
    %\hline
    AutoSA \cite{wang2021autosa} & Dense MM, etc\tnote{1} & $4\times10^6$ & $7\times10^9$ &
    950 GFLOP/s & \textbf{Yes} & No & \textbf{Yes} & No \\

    %\hline
    \cite{fowers2014high} & SpMV & $5\times10^6$ & $<1\times10^7$ &
    3.9 GFLOP/s & \textbf{Yes} & No & \textbf{Yes} & No \\

    %\hline
    Spaghetti \cite{hojabr2021spaghetti} & SpGEMM & $1.6\times10^7$ & - &
    27 GFLOP/s & \textbf{Yes} & No & \textbf{Yes} & No \\

    %\hline
    Tensaurus \cite{srivastava2020tensaurus} & SpMV, SpMM, etc\tnote{2} & $4.2\times10^6$ & - &
    512 GFLOP/s\tnote{3} & No & \textbf{Yes} & No & No \\
    
    %\hline
    ExTensor \cite{hegde2019extensor} & SpMM, SpGEMM, etc\tnote{2} & $6\times10^6$ & - &
    64 GFLOP/s & No & \textbf{Yes} & No & No \\
    
    %\hline
    SIGMA \cite{qin2020sigma} & SpGEMM & - & - &
    - & No & \textbf{Yes} & No & No \\

    %\hline
    SpArch \cite{zhang2020sparch} & SpGEMM & $1.65\times10^7$ & - &
    10.4 GFLOP/s & No & \textbf{Yes} & No & No \\

    %\hline
    OuterSPACE \cite{pal2018outerspace} & SpGEMM & $1.65\times10^7$ & - &
    2.9 GFLOP/s & No & \textbf{Yes} & No & No \\

    %\hline
    SpaceA \cite{xie2021spacea} & SpMV & $1.4\times10^7$ & $1.43\times10^7$ &
    - & No & \textbf{Yes} & No & No \\
    
    %\hline
    \sextansFPGA & SpMM & $3.7\times10^7$ & $3\times10^{10}$ &
    190.5 GFLOP/s & No & \textbf{Yes} & No & \textbf{Yes} \\
    
    %\hline
    \sextansASIC & SpMM & $3.7\times10^7$ & $3\times10^{10}$ &
    1288 GFLOP/s & \textbf{Yes} & No & \textbf{Yes} & \textbf{Yes} \\
    \hline
  \end{tabular}

  \begin{tablenotes}
        \footnotesize
        \item[1] Other dense tensor kernels such as TTMc, MTTKRP are also supported. $^2$ Other dense tensor kernels such as sparse TTM, sparse TTV are also supported.
        \item[3] 512 GFLOP/s is achieved on dense multiplication, and the throughput of sparse multiplication is lower.  
      \end{tablenotes}
    \end{threeparttable}
  
\end{tableA*}
